# Supplementary material for: Text is NOT Enough: Integrating Visual Impressions into Open-domain Dialogue Generation
Source: arXiv:2109.05778 source file (2021-09-18)
Supplement: Supplementary file 1 [file appendix.tex]

\section{Human Evaluation on \textit{PersonaChat}}

\begin{table}[h]
\small
\centering
\begin{tabular}{lrrrr}
  \toprule[1pt] 
  \textbf{Opponent} & \textbf{Win} & \textbf{Loss} & \textbf{Tie} & \textbf{Kappa} \\
  \hline
  VisAD vs. SEQ2SEQ & 57\% & 20\% & 23\% & 0.604 \\
  VisAD vs. CVAE & 45\% & 27\% & 28\% & 0.468 \\
  VisAD vs. DialogWAE & 53\% & 21\% & 29\% & 0.540\\
  VisAD vs. Transformer & 40\% & 31\% & 29\% & 0.427\\
  VisAD vs. GVT & 48\% & 27\% & 25\% & 0.506 \\
  VisAD vs. VD-BERT & 55\% & 19\% & 26\% & 0.559 \\
  \bottomrule[1pt]
\end{tabular}
\caption{The results of human evaluation on  \textit{PersonaChat} datasets.}
\label{tab:human_persona}
\end{table}

\section{Ablation Study on \textit{PersonaChat}}

\begin{table}[h]
% \small
\centering
\resizebox{0.48\textwidth}{10mm}{
\begin{tabular}{lccccccc}
\toprule[1pt]
 \textbf{Model} & \textbf{PPL} & \textbf{B} & \textbf{D1} & \textbf{D2} & \textbf{Avg} & \textbf{Ext} & \textbf{Gre} \\
  \hline
   (a) \textit{w/o} IM & 25.65 & 4.31  & \textbf{6.11} & 21.85 & 57.82 & 37.98 & 48.06 \\
   (b) \textit{w/o} KW & 27.81 & 4.59  & 5.63 & 23.04 & 56.02 & 37.71 & 44.52 \\
   (c) \textit{w/o} KAL & 29.47 & 4.30  & 5.42 & 22.66 & 54.29 & 36.14 & 46.85   \\
   \textbf{Full Model} & \textbf{19.58} & \textbf{5.03}  & {6.08} & \textbf{26.52} & \textbf{59.60} & \textbf{40.03} & \textbf{50.96}   \\
\bottomrule[1pt]
\end{tabular}}
\caption{Ablation results on  \textit{PersonaChat} datasets. ``IM'' refers to the image representation, ``KW'' refers to the keyword information, ``KAL'' refers to the auxiliary keyword loss.}
\label{tab:ablation_personachat}
\end{table}
